# Supplementary material for: Benanza: Automatic $\mu$Benchmark Generation to Compute "Lower-bound" Latency and Inform Optimizations of Deep Learning Models on GPUs
Source: arXiv:1911.06922 source file (2020-02-19)
Supplement: Supplementary file 1 [file 9-appendix.tex]

\subsection{Plot of Critical Path of Inception-v1}

\begin{figure}
	\centering
	\resizebox{.08\totalheight}{!}{
		\includegraphics[width=0.48\linewidth]{fig/inception_v1_parallel.pdf}
	}
	\caption{The full critical path of \texttt{Inception-V1} on a Tesla\_V100 system with batch size 1}
	\label{fig:inception_full}
\end{figure}
